# Supplementary material for: Multiple origins of extra electron diffractions in fcc metals
Source: arXiv:2311.10326 ancillary file (2023-11-17)
Supplement: Supplementary file 1 [file si.pdf]

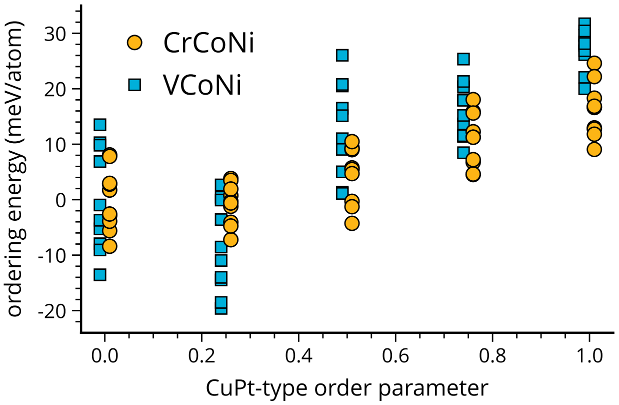


Supplementary Figure 1: Ab initio-calculated energies of CrCoNi and VCoNi configurations containing CuPt-type ($L1_1$) Cr or V concentration waves with amplitudes defined by an order parameter following the formalism of Ref. [1]. A value of 0 indicates random solid solutions, which define reference energies, while the maximum value of 1 corresponds to the complete segregation of V or Cr onto alternating $(\bar{1}1\bar{1})$, and simultaneously $(31\bar{1})$, planes. This type of concentration wave, which directly equates to diffuse intensity in the mean-field picture of scattering [1], largely raises energies relative to random alloys. The slightly negative VCoNi ordering energy associated with a parameter of 0.25 is not significant enough to promote meaningful chemical rearrangement, particularly when chemically equilibrated structures minimizing V-V nearest neighbors are an order of magnitude more favorable [2]. Collinearly spin-polarized density-functional calculations were performed using the Vienna Ab initio Simulation Package (VASP) [3] with a plane-wave [4, 5] energy cutoff of 520 eV and a linear k-point density of 0.15 Å. Geometrically optimized structures contained 24 atoms divided between two $(\bar{1}1\bar{1})$ planes according to the order parameter. In order to minimize variability, the distribution of nearest neighbor pairs in all calculations, which is unaffected by CuPt-type concentration waves, was constrained to that of a random solution.

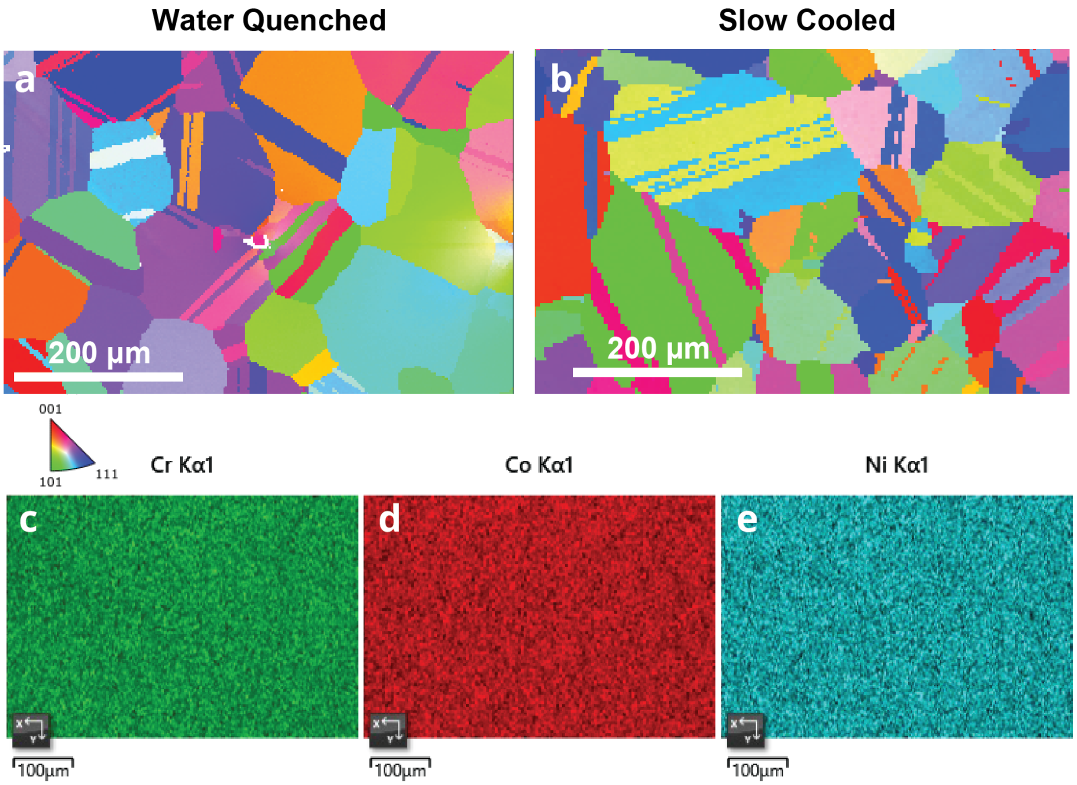


Supplementary Figure 2: Typical recrystallized CrCoNi microstructure with equiaxed grains, annealing twins, and no apparent chemical segregation. EBSD-inverse pole figure (IPF) color maps of the initial microstructure are given for (a) water-quenched and (b) slow-cooled CrCoNi samples. (c-e) show representative EDS maps of water-quenched and slow-cooled CrCoNi samples. The initial microstructure of the CrCoNi alloy was determined by electron backscatter diffraction (EBSD) and energy-dispersive x-ray spectroscopy (EDS) on an FEI Scios 2 DualBeam FIB/SEM under an operating voltage of 20 kV and a current of 13 nA. The EBSD scans have a field of view of $594 \times 40$ μm and a step size of 2.3 μm for quenched samples, and those of $1040 \times 715$ μm and 4 μm for slow-cooled CrCoNi, respectively. Raw EBSD data were post-processed using the AztecCrystal software using a procedure similar to that described in Ref. [6]. The initial microstructure of CrCoNi is a single fcc phase with grain sizes of $83 \pm 47$ μm and $93 \pm 49$ μm for quenched and slow-cooled samples, respectively. The overall composition was confirmed to be near equiatomic.

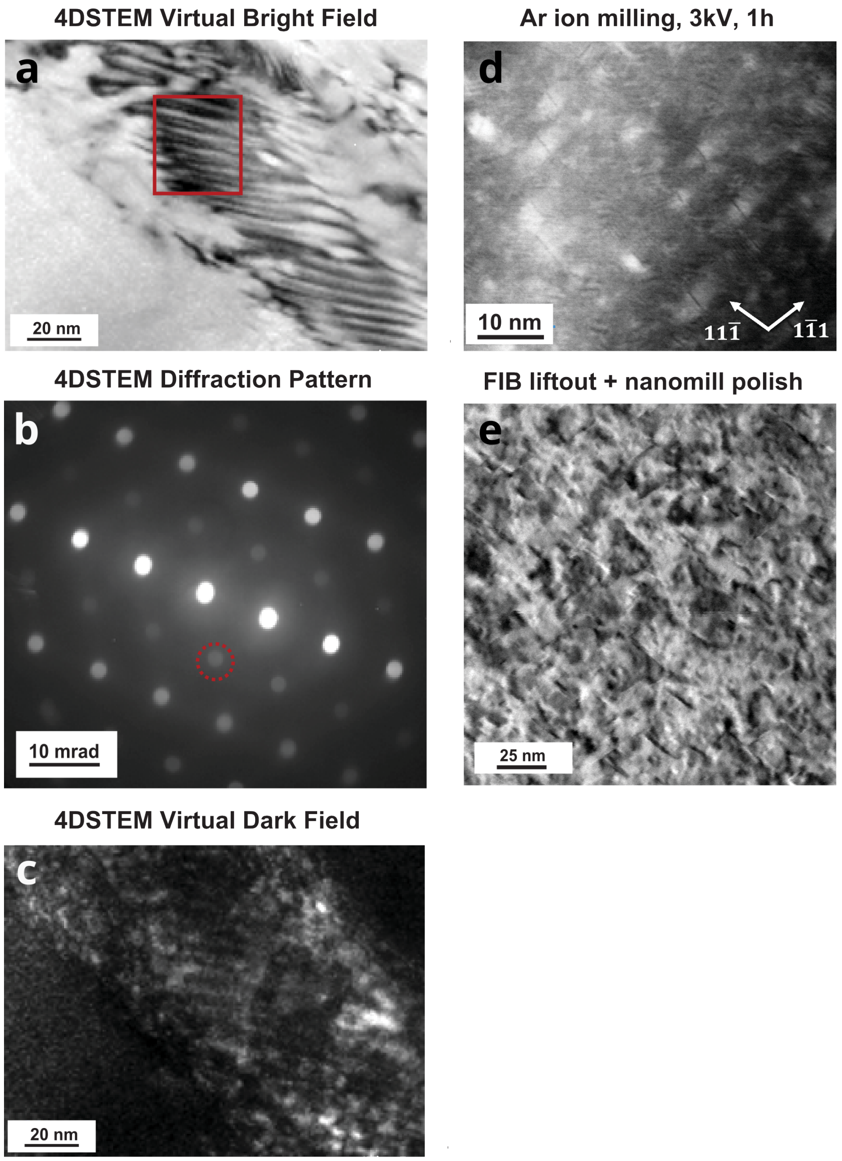


Supplementary Figure 3: SFs from mechanical deformation: (a) Reconstructed 4DSTEM virtual bright-field image of a slightly deformed CrCoNi sample showing a shear band consisting of separated Shockley partial dislocations imaged near the [$\bar{1}$12] ZA; (b) the sum of the DPs for pixels in the red boxed area shown in (a); (c) 4DSTEM virtual dark-field image of the same area using the red circle in (b) as the virtual aperture. The $\frac{1}{2}\{311\}$ superlattice peaks are clearly correlated to the stacking faults between Shockley partial dislocations. SFs from ion milling: (d) STEM-LAADF image of an electropolished CrCoNi sample followed by Ar ion milling at a low voltage of 3 kV for 1 h; (e) STEM-BF image of a CrCoNi FIB lamella polished at 2 kV Ga+ beam followed by 900 V and 500 V nanomilling. The imaging was performed in the $\vec{g} = [200]$ 2-beam condition near the [110] ZA. The edge-on Franks loops are projected as short straight lines on the (11$\bar{1}$) and (1$\bar{1}$1) planes perpendicular to the (11$\bar{1}$) and (1$\bar{1}$1) g-vectors. Although care has been taken to mitigate the damage caused by Ar and Ga ions (e.g., Ar ion milling was done under a low gun angle of $\pm 3°$ and a low voltage of 3 kV, and FIB was finished by a 2 kV polish followed by 900 V and 500 V nanomilling), large amounts of Frank loops were detected by our TEM characterization, as shown in (d, e), which will result in the aforementioned superlattice peaks in the DP. The pervasive existence of well-defined Frank loops after ion milling is not seen in conventional fcc metals, where ion beam damage only leads to smaller vacancy/interstitial clusters shown as black dots or black-white contrast under TEM [7]. The prevalence of Frank loops in $3d$ solid solutions is likely related to their low stacking fault energies.

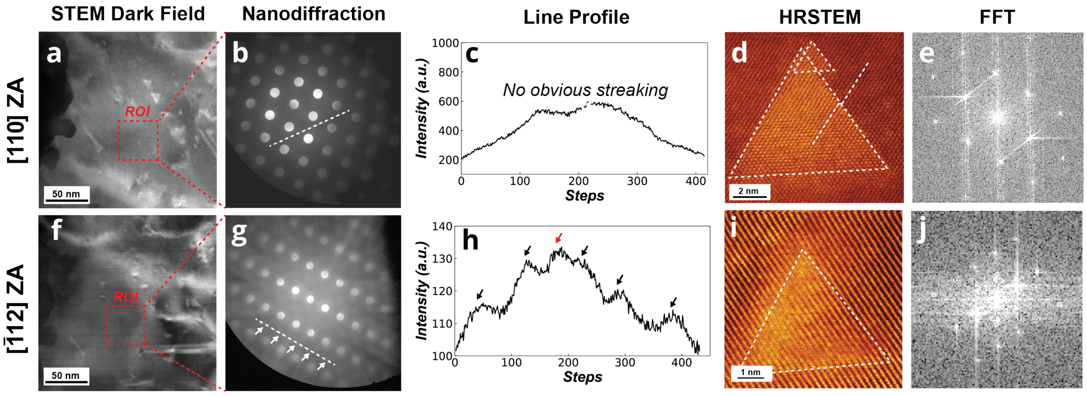


Supplementary Figure 4: SFTs are formed by the local agglomeration of vacancies into triangular platelets during rapid cooling. This phenomenon is particularly apparent at ultra-high cooling rates, such as those achieved by additive manufacturing, which can produce 20–50 nm SFTs that are readily visible in STEM-BF [8]. Here, less visible SFTs are shown to form in water-quenched CrCoNi. (a) STEM-DF image of a 20–50 nm thick region (left-to-right) in a quenched CrCoNi sample along the [110] ZA; (b) summed nanodiffraction pattern from the red boxed region in (a), which is free of obvious stacking faults; (c) the intensity profile of the dashed line marked in (b), showing no obvious streaking; (d) atomic-resolution STEM-LAADF image from the quenched CrCoNi sample, showing a $\sim$10 nm SFT where the change of stacking sequence can be directly resolved and a smaller $\sim$2 nm SFT; (e) the Fourier transform of (d), showing clear streaking; and (f-j) the same information as in (a-e) for the same region in the sample along the [$\bar{1}$12] ZA. The line profile given in (h) shows clear diffuse $\frac{1}{2}\{311\}$ superlattice peaks, as indicated by the black arrows. The red arrow results from the intensity of a Kikuchu band. The Fourier transform of the SFT viewed along [$\bar{1}$12] ZA given in (j) also shows a $\frac{1}{2}\{311\}$ superlattice.

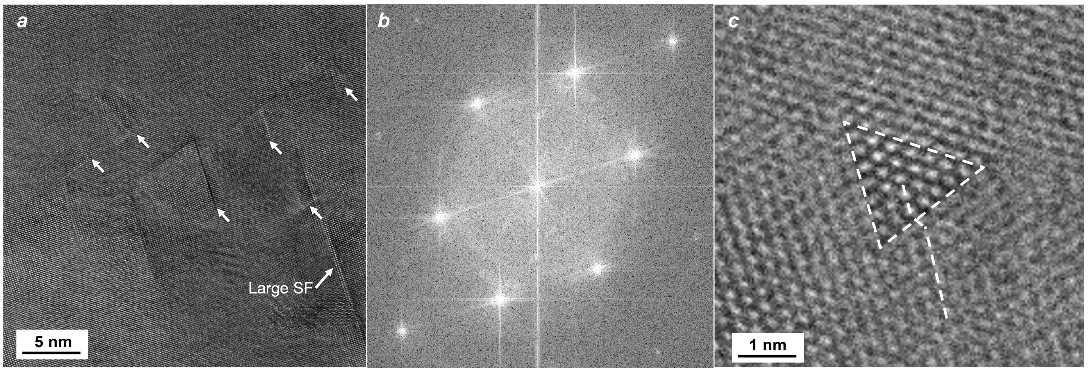


Supplementary Figure 5: (a) Image-corrected HRTEM image of a 20–30 nm thick region in a quenched CrCoNi sample along the [110] ZA showing a number of small SFTs and a large SF, indicated by arrows; (b) is the FFT of (a) showing clear streaking from the SF and SFTs; and (c) zoomed-in view of a small SFT ($\sim$2 nm), where the change in the stacking sequence can be directly resolved.

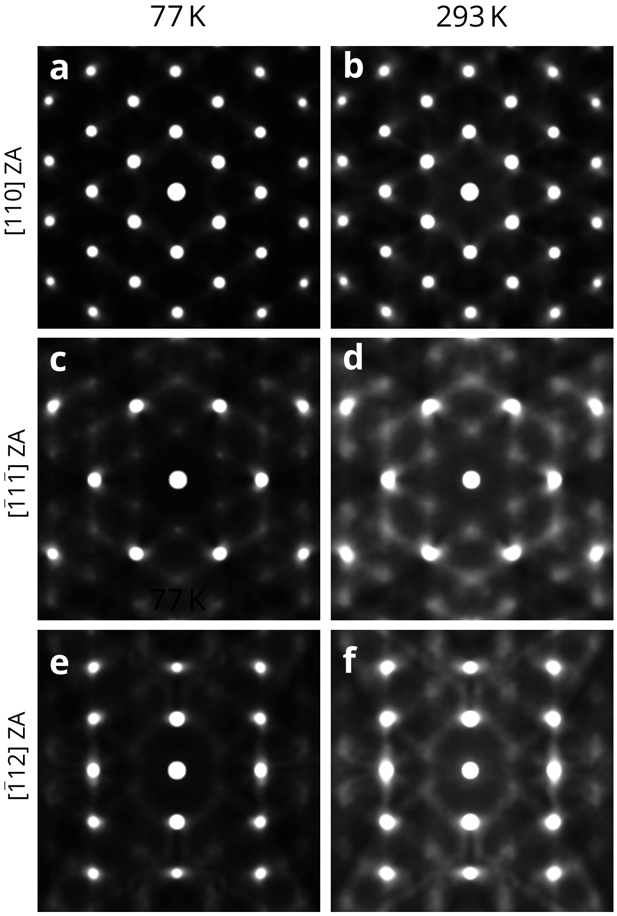


Supplementary Figure 6: Extra diffractions from thermal scattering in Cu. (See Fig. 1 for coordinates.) Multislice DPs for 30 nm-thick MD simulations at 77 K and 293 K in the (a,b) [110], (c,d) $[\bar{1}12]$, and (e,f) $[\bar{1}1\bar{1}]$ ZAs. While only minimal streaking appears in the [110] ZA in (a,b), clear extra diffractions emerge at 293 K in both the (d) $[\bar{1}1\bar{1}]$ and (f) $[\bar{1}12]$ ZAs. The latter intensities lie near $\frac{1}{2}\{311\}$, but actually curve inward away from the origin, just as in the experimental DP of Ref. [9]. Thermal diffuse intensities remain faintly visible in (c) and (e). Cu was modeled using the atomic cluster expansion [10] described in Ref. [11].

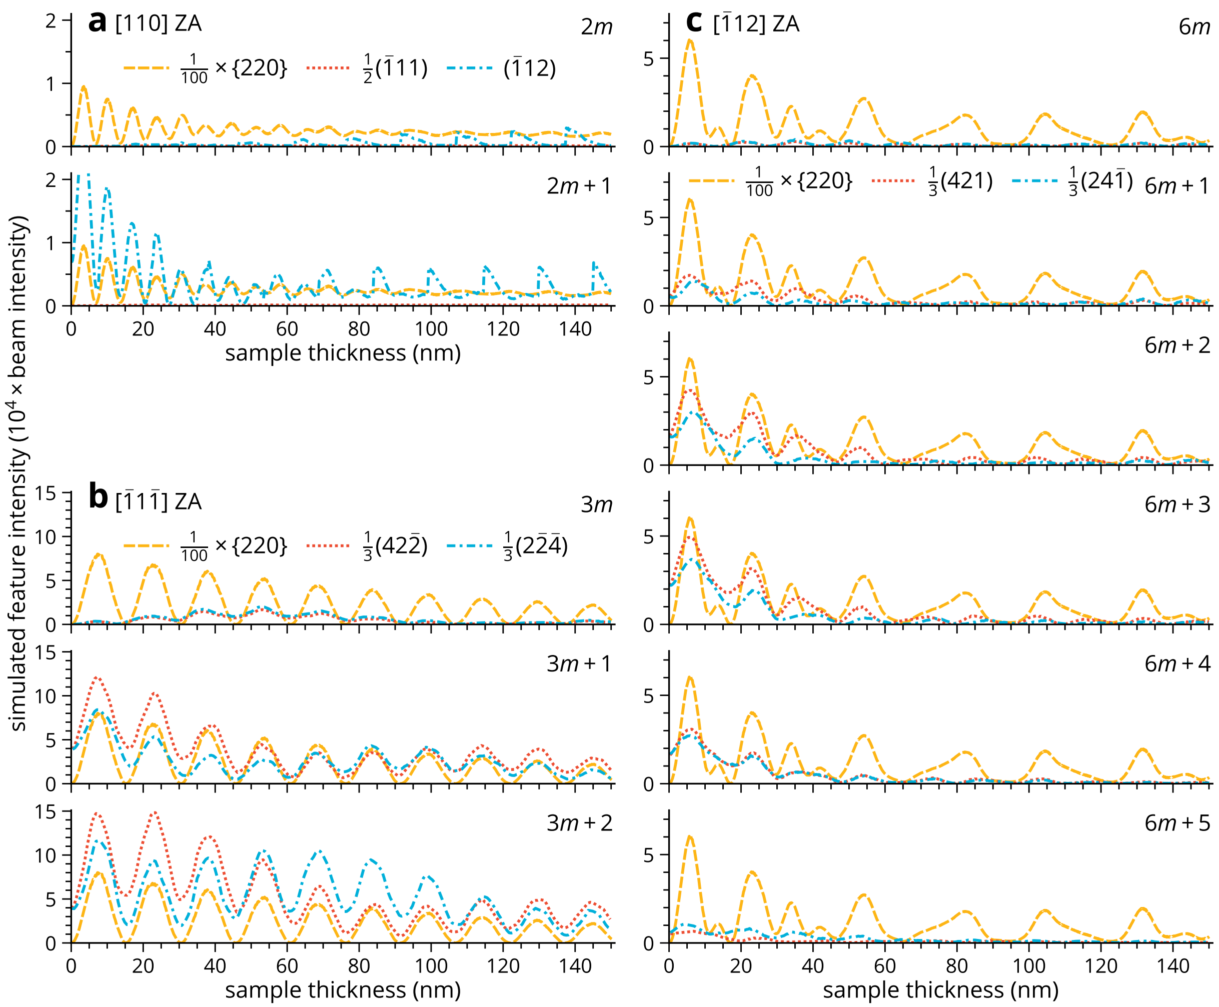


Supplementary Figure 7: Simulated extra diffraction intensities for individual stacking terminations in Ni. The number of layers in each configuration is noted as a multiple of some integer $m$, corresponding to perfectly commensurate stacking sequences, plus some number of incommensurate layers giving rise to extra diffractions. (a) Calculations for the [110] ZA, comparing $\{220\}$ diffractions at one hundredth scale to negligible $\frac{1}{2}\{111\}$ intensities that would reflect any streaking. Dynamical/surface scattering causes other features further from the origin. (b) Equivalent results for the $[\bar{1}1\bar{1}]$ ZA, where two types of extra diffractions occur. (c) Calculations for the six possible terminations of the $[\bar{1}12]$ ZA, highlighting two of the brightest extra diffractions, which are near but distinct from experimentally observed $\frac{1}{2}\{311\}$ intensities.

## References


[1] A. G. Khachaturyan, *Theory of Structural Transformations in Solids* (Dover, Mineola, 2008).

[2] X. Chen *et al.*, Nature **592**, 712 (2021).

[3] G. Kresse and J. Hafner, Phys. Rev. B **47**, 558 (1993).

[4] G. Kresse and J. Furthmüller, Phys. Rev. B **54**, 11169 (1996).

[5] G. Kresse and J. Furthmüller, Comput. Mater. Sci. **6**, 15 (1996).

[6] M. Zhang *et al.*, Acta Mater. **241**, 118380 (2022).

[7] M. L. Jenkins and M. A. Kirk, *Characterisation of Radiation Damage by Transmission Electron Microscopy* (CRC, Boca Raton, 2000).

[8] T. M. Smith *et al.*, Nature **617**, 513 (2023).

[9] L. Li *et al.*, Acta Mater. **243**, 118537 (2023).

[10] R. Drautz, Phys. Rev. B **99**, 014104 (2019).

[11] Y. Lysogorskiy *et al.*, npj Comput. Mater. **7**, 97 (2021).
